# Supplementary material for: Certified Defense via Latent Space Randomized Smoothing with Orthogonal Encoders
Source: arXiv:2108.00491 source file (2021-08-01)
Supplement: Supplementary file 2 [file supp_packages.tex]

\usepackage{url}
\usepackage{dsfont}
\usepackage{xspace}
%\usepackage{hyperref}
%\usepackage{times}
% \usepackage[authoryear]{natbib}
% \usepackage[square,sort,comma,numbers]{natbib}
\usepackage{natbib}
%\usepackage[outdir=./]{epstopdf}
\usepackage{graphicx,float,pgfplots,wrapfig,sidecap,lipsum}
\usepackage{tabularx}
\usepackage{booktabs}
\usepackage{paralist}

% \usepackage{algorithm}
% \usepackage{algorithmic}
% \usepackage{algpseudocode}
% \newcommand{\theHalgorithm}{\arabic{algorithm}}
% \usepackage[linesnumbered,algoruled,boxed,lined]{algorithm2e}
% \usepackage{algorithmicx}
% \usepackage{algpseudocode}
%\usepackage[pass]{geometry}
\usepackage{amsfonts}
\usepackage{amsthm}
\usepackage{amsmath}
\usepackage{amssymb}
\usepackage{enumitem}
\usepackage{xcolor}
\usepackage[font=normal,labelfont=bf]{caption}
\usepackage{mathtools} 
\usepackage{bbm}
\usepackage{multirow}

\usepackage{tablefootnote}
%\usepackage{subfig}
\usepackage{subcaption}
\usepackage{subfloat}
% \usepackage{hyperref,psfrag} % not allowed by AAAI
\usepackage{tikz}
\usetikzlibrary{fit}
\usetikzlibrary{calc,shapes}
\usetikzlibrary{decorations.pathmorphing} % noisy shapes
\usetikzlibrary{fit}					% fitting shapes to coordinates
\usetikzlibrary{backgrounds}	% drawing the background after the foreground

% \usepackage{refcheck}

\usepackage{bm}
\usepackage{mathrsfs} 
%\usepackage{fourier}
\usepackage{stmaryrd}
\usepackage[utf8]{inputenc}
\usepackage[english]{babel}
\usepackage{diagbox}

%pgfplots
\usepackage[utf8]{inputenc}
% \usepackage{fontspec}  % optional
\usepackage{pgfplots}
\pgfplotsset{compat=newest}
\usepgfplotslibrary{groupplots}
\usepgfplotslibrary{dateplot}
